# Supplementary material for: Simple High-Bandwidth Sideband Locking with Heterodyne Readout
Source: arXiv:1610.01631 source file (2016-10-05)
Supplement: Supplementary file 1 [file Supplementary_Materials.pdf]

# Supplementary Information for "Simple High-Bandwidth Sideband Locking with Heterodyne Readout"

October 5, 2016

## Contents


**1 Reflection from a high-finesse asymmetric cavity** **1**

**2 Shorthand notation** **2**

**3 Transfer function from laser noise to error signal** **2**

3.1 Case 1: Frequency noise only, ideal EOM, cavity resonant with carrier . . . . . . . . . . . . . . . . . . 4

3.2 Case 2: Frequency noise only, ideal EOM, cavity resonant with upper sideband . . . . . . . . . . . . 5

3.3 Case 3: Amplitude noise only, ideal EOM, cavity resonant with carrier . . . . . . . . . . . . . . . . . . 5

3.4 Case 4: Amplitude noise only, ideal EOM, cavity resonant with upper sideband . . . . . . . . . . . . 5

**4 Transfer from VCO input to error signal** **6**

**5 Error signal for wider range of VCO outputs** **7**


# 1 Reflection from a high-finesse asymmetric cavity

Consider a cavity of length $L$ with mirrors that are not identical, having field transmission coefficients $it_1$ and $it_2$ and reflection coefficients $-r_1$ and $-r_2$ (where $t_i$ and $r_i$ are real positive and $|t_i|^2 + |r_i|^2 \leq 1$). If the first mirror is driven by a field of amplitude $E_{in}$ and angular frequency $\omega$, the steady-state reflected field – a sum of the prompt reflection and all subsequent paths leaking from the input mirror – can be calculated from the resulting geometric series:

$$\begin{aligned} E_r &= E_{in}\left[-r_1 + t_1^2 r_2 e^{-2i\omega L/c} + t_1^2 r_2 e^{-2i\omega L/c} r_1 r_2 e^{-2i\omega L/c} + t_1^2 r_2 e^{-2i\omega L/c}\left(r_1 r_2 e^{-2i\omega L/c}\right)^2 + ...\right] \\ &= E_{in}\left[-r_1 + \frac{t_1^2 r_2 e^{-2i\omega L/c}}{1 - r_1 r_2 e^{-2i\omega L/c}}\right] \end{aligned} \quad (1)$$

In the high-finesse limit, this can be expanded in terms of the small transmission coefficients $t_i \ll 1$ and loss coefficients $\rho_i \equiv \sqrt{1 - r_i^2} \ll 1$. The second term in the expression for $E_r$ is then

$$\frac{t_1^2 r_2 e^{-i2\omega L/c}}{1 - r_1 r_2 e^{-i2\omega L/c}} \approx \frac{t_1^2}{\frac{1}{2}\rho_2^2 + \frac{1}{2}\rho_1^2 + i\frac{2L\delta}{c}} \quad (2)$$

where we introduce the detuning $\delta = \omega - \omega_r$ from the $n^{\text{th}}$ cavity resonance frequency $\omega_r = nc/2L$, and assume the detuning is also small relative to the mode spacing $c/2L$. Combining this with Eqs. 1 and 2,

$$E_r = E_{in}\left[\frac{t_1^2 \tau c/L}{1 + i2\tau\delta} - r_1\right] \quad (3)$$

where $\tau = \frac{2L/c}{\rho_1^2 + \rho_2^2}$ is the power ringdown time of the cavity.

## 2 Shorthand notation

The following sections contain a lot of bookkeeping. To save space and typos, we adopt the following shorthand notation

$$\begin{aligned} C_a, S_a &\equiv \cos(\omega_a t), \sin(\omega_a t) \\ C_{a\pm b}, S_{a\pm b} &\equiv \cos(\omega_a t \pm \omega_b t), \sin(\omega_a t \pm \omega_b t) \\ C_{a\pm b\psi}, S_{a\pm b\psi} &\equiv \cos(\omega_a t \pm (\omega_b t + \psi)), \sin(\omega_a t \pm (\omega_b t + \psi)) \\ C_{a\pm 2b\psi}, S_{a\pm 2b\psi} &\equiv \cos(\omega_a t \pm (2\omega_b t + \psi)), \sin(\omega_a t \pm (2\omega_b t + \psi)) \end{aligned}$$

As a matter of algebraic taste, we save complex notation for the end (the diode and mixers both involve nonlinear operations).

## 3 Transfer function from laser noise to error signal

In this section, we add a small, steady-state classical "noise" term to the field from a laser, and then propagate this through the electro-optical modulator (EOM), cavity, photodiode, and mixers to determine our system's overall transfer function.

Suppose the laser has a "noise" component at frequency $\omega_n$, with amplitude modulation of the form

$$\epsilon(t) = \epsilon_n \cos(\omega_n t)$$

for constant $\epsilon_n$ and frequency modulation of the form

$$\Omega(t) = \Omega_n \cos(\omega_n t)$$

for constant depth $\Omega_n$. In this case, the field (nominally of the noiseless form $\sqrt{P_l}\cos(\omega_l t)$ for laser frequency $\omega_l$ and power $P_l$) is

$$E(t) = \sqrt{P_l}(1 + \epsilon_n C_n)\cos(\omega_l t + \phi_n S_n)$$

where

$$\phi_n \equiv \Omega_n/\omega_n \tag{4}$$

is the phase noise amplitude. If this laser passes through an electro-optical modulator (EOM) driven by a voltage-controlled oscillator (VCO) voltage of the form

$$V_{VCO}(t) = V_e \sin(\omega_e t)$$

with constant amplitude $V_e$ and frequency $\omega_e$, $E$ is further modified to

$$E(t) = \sqrt{P_l}(1 + \epsilon_n C_n + \epsilon_e S_e)\cos(\omega_l t + \phi_n S_n + \phi_e S_e), \tag{5}$$

where $\phi_e = \eta_{EOM} V_{VCO}$ is the phase excursion for a "flat" EOM conversion efficiency $\eta_{EOM}$ (units of rad/V), and we have included a small amount of "accidental" amplitude modulation $\epsilon_e$ due to imperfections in the EOM optics. If we assume the modulations are small ($\epsilon_n, \epsilon_e, \phi_n, \phi_e \ll 1$), the field can be Taylor expanded to second order in these quantities and rewritten in terms of a carrier at $\omega_l$ and 12 sidebands:

$$\begin{aligned} \frac{E(t)}{\sqrt{P_l}} \approx & \left(1 - \frac{1}{4}\phi_e^2 - \frac{1}{4}\phi_n^2\right) C_l \\ & + \frac{1}{2}\epsilon_n (C_{l+n} + C_{l-n}) + \frac{1}{2}\phi_n (C_{l+n} - C_{l-n}) \\ & + \frac{1}{2}\epsilon_e (S_{l+e} - S_{l-e}) + \frac{1}{2}\phi_e (C_{l+e} - C_{l-e}) \\ & + \frac{1}{8}\phi_n^2 (C_{l+2n} + C_{l-2n}) + \frac{1}{4}\phi_n\epsilon_n (C_{l+2n} - C_{l-2n}) \\ & + \frac{1}{8}\phi_e^2 (C_{l+2e} + C_{l-2e}) + \frac{1}{4}\phi_e\epsilon_e (-2S_l + S_{l+2e} + S_{l-2e}) \\ & + \frac{1}{4}\phi_e\phi_n (C_{l+e+n} - C_{l+e-n} - C_{l-e+n} + C_{l-e-n}) \\ & + \frac{1}{4}\phi_n\epsilon_e (S_{l+e+n} - S_{l+e-n} - S_{l-e+n} + S_{l-e-n}) \\ & + \frac{1}{4}\phi_e\epsilon_n (C_{l+e+n} + C_{l+e-n} - C_{l-e+n} - C_{l-e-n}). \end{aligned} \tag{6}$$

Now suppose these beams land on a cavity with either a cavity mode "$A$" resonant with the *carrier* at $\omega_l$ or a cavity mode "$B$" resonant with the *upper sideband* at $\omega_l + \omega_e$ (we will track both options through the calculation, allowing us to choose different scenarios at the end). In the limit where the noise frequency is comparable to the cavity ringdown time ($\omega_n \sim 1/\tau$) and the VCO frequency is comparatively "high" ($\omega_e \gg 1/\tau$), only the red terms will interact with resonance $A$ and only the blue terms interact with resonance $B$. According to Eq. 3, cavity mode $X$ has reflection coefficient

$$\begin{aligned} r_X(\delta) &\approx -r_1\rho_X(\delta) \\ \rho_X(\delta) &\equiv 1 - \frac{t_1^2\tau c/L}{1+i2\tau\delta} \end{aligned} \tag{7}$$

for cavity parameters $r_1$, $t_1$, and $\tau$, (all real positive) and detuning $\delta$. As a result, the field reflected from the cavity will be

$$\begin{aligned} \frac{-E(t)}{r_1\sqrt{P_l}} = & \left(1 - \frac{1}{4}\phi_e^2 - \frac{1}{4}\phi_n^2\right)\rho_{A0}C_l \\ & + \frac{1}{2}\epsilon_n\left(\rho_{An}C_{l+n\psi_A} + \rho_{An}C_{l-n\psi_A}\right) + \frac{1}{2}\phi_n\left(\rho_{An}C_{l+n\psi_A} - \rho_{An}C_{l-n\psi_A}\right) \\ & + \frac{1}{2}\epsilon_e\left(\rho_{B0}S_{l+e} - \alpha S_{l-e}\right) + \frac{1}{2}\phi_e\left(\rho_{B0}C_{l+e} - \alpha C_{l-e}\right) \\ & + \frac{1}{8}\phi_n^2\left(\rho_{A2n}C_{l+2n\phi_A} + \rho_{A2n}C_{l-2n\phi_A}\right) + \frac{1}{4}\phi_n\epsilon_n\left(\rho_{A2n}C_{l+2n\phi_A} - \rho_{A2n}C_{l-2n\phi_A}\right) \\ & + \frac{1}{8}\phi_e^2\left(C_{l+2e} + C_{l-2e}\right) + \frac{1}{4}\phi_e\epsilon_e\left(-2S_l + S_{l+2e} + S_{l-2e}\right) \\ & + \frac{1}{4}\phi_e\phi_n\left(\rho_{Bn}C_{l+e+n\psi_B} - \rho_{Bn}C_{l+e-n\psi_B} - \alpha C_{l-e+n} + \alpha C_{l-e-n}\right) \\ & + \frac{1}{4}\phi_n\epsilon_e\left(\rho_{Bn}S_{l+e+n\psi_B} - \rho_{Bn}S_{l+e-n\psi_B} - \alpha S_{l-e+n} + \alpha S_{l-e-n}\right) \\ & + \frac{1}{4}\phi_e\epsilon_n\left(\rho_{Bn}C_{l+e+n\psi_B} + \rho_{Bn}C_{l+e-n\psi_B} - \alpha C_{l-e+n} - \alpha C_{l-e-n}\right). \end{aligned} \tag{8}$$

where we define

$$\begin{aligned} \rho_{X0} &\equiv \rho_X(0) \\ \rho_{Xn} &\equiv |\rho_X(\omega_n)| \\ \psi_X &\equiv \arg\left[\rho(\omega_n)\right] = -\arg\left[\rho(-\omega_n)\right] \\ \rho_{X2n} &\equiv |\rho_X(2\omega_n)| \\ \phi_X &\equiv \arg\left[\rho(2\omega_n)\right] = -\arg\left[\rho(-2\omega_n)\right] \end{aligned}$$

to indicate the magnitude and phase changes from the two cavity modes upon reflection,[1] and we have attached a prefactor $\alpha = 1$ to all the terms having frequencies near the *lower* sidebands to "track" the effect of the lower sideband on the resulting demodulated signal (see below).

When all of this light lands on an amplified photodiode, the voltage it produces comprises all frequencies generated by the quantity $E^2(t)$ that are within the diode's electronic bandwidth (a few GHz in our case). Additionally, anticipating the subsequent demodulation at $\omega_e$ and our eventual interest only in the noise term at $\omega_n$, we can ignore the *vast* majority of these terms. Assuming a "flat" photodiode conversion efficiency $\eta_{PD}$ (units of V/W) and again keeping only terms up to second order in $\epsilon_n, \epsilon_e, \phi_n, \phi_e$, its output voltage $V_{PD}(t)$ is then given by

$$\begin{aligned} \frac{2V_{PD}(t)}{\eta_{PD}r_1^2P_l} \approx & \ldots + \rho_{A0}C_l\phi_e\phi_n\left(\rho_{Bn}C_{l+e+n\psi_B} - \rho_{Bn}C_{l+e-n\psi_B} + \alpha C_{l-e-n} - \alpha C_{l-e+n}\right) \\ & + \rho_{A0}C_l\phi_n\epsilon_e\left(\rho_{Bn}S_{l+e+n\psi_B} - \rho_{Bn}S_{l+e-n\psi_B} - \alpha S_{l-e+n} + \alpha S_{l-e-n}\right) \\ & + \rho_{A0}C_l\phi_e\epsilon_n\left(\rho_{Bn}C_{l+e+n\psi_B} + \rho_{Bn}C_{l+e-n\psi_B} - \alpha C_{l-e+n} - \alpha C_{l-e-n}\right) \\ & + \epsilon_n\left(\rho_{An}C_{l+n\psi_A} + \rho_{An}C_{l-n\psi_A}\right)\left[\epsilon_e\left(\rho_{B0}S_{l+e} - \alpha S_{l-e}\right) + \phi_e\left(\rho_{B0}C_{l+e} - \alpha C_{l-e}\right)\right] \\ & + \phi_n\left(\rho_{An}C_{l+n\psi_A} - \rho_{An}C_{l-n\psi_A}\right)\left[\epsilon_e\left(\rho_{B0}S_{l+e} - \alpha S_{l-e}\right) + \phi_e\left(\rho_{B0}C_{l+e} - \alpha C_{l-e}\right)\right] \end{aligned}$$

[1] Note $-1 < \rho_X(0) < 1$, depending on the cavity parameters.

or, expanding to single frequencies,

$$\begin{aligned}\frac{4V_{PD}(t)}{\eta_{PD}r_1^2P_l} \approx\ & ... + \rho_{A0}\phi_e\phi_n\left(\rho_{Bn}C_{e+n\psi_B} - \rho_{Bn}C_{e-n\psi_B} + \alpha C_{e+n} - \alpha C_{e-n}\right) \\ & + \rho_{A0}\epsilon_e\phi_n\left(\rho_{Bn}S_{e+n\psi_B} - \rho_{Bn}S_{e-n\psi_B} + \alpha S_{e-n} - \alpha S_{e+n}\right) \\ & + \rho_{A0}\phi_e\epsilon_n\left(\rho_{Bn}C_{e+n\psi_B} + \rho_{Bn}C_{e-n\psi_B} - \alpha C_{e-n} - \alpha C_{e+n}\right) \\ & + \rho_{An}\epsilon_e\epsilon_n\left(\rho_{B0} + \alpha\right)\left(S_{e-n\psi_A} + S_{e+n\psi_A}\right) \\ & + \rho_{An}\phi_e\epsilon_n\left(\rho_{B0} - \alpha\right)\left(C_{e-n\psi_A} + C_{e+n\psi_A}\right) \\ & + \rho_{An}\epsilon_e\phi_n\left(\rho_{B0} - \alpha\right)\left(S_{e-n\psi_A} - S_{e+n\psi_A}\right) \\ & + \rho_{An}\phi_e\phi_n\left(\rho_{B0} + \alpha\right)\left(C_{e-n\psi_A} - C_{e+n\psi_A}\right)\end{aligned} \tag{9}$$

At this point, we can demodulate this signal with the VCO signal $\sim \sin(\omega_e t)$ to produce the "classic" Pound-Drever-Hall (PDH) error signal quadrature $V_Y$, and we can demodulate with a phase-shifted signal $\sim \cos(\omega_e t)$ to produce the other quadrature $V_X$. Assuming a "flat" mixer efficiency $\eta_M$, (i.e. $V_Y = \eta_M V_{PD} S_e$ and $V_X = \eta_M V_{PD} C_e$) and keeping only terms at $\omega_n$, the two quadratures simplify to

$$\begin{aligned}\frac{4V_Y(t)}{\eta_M\eta_{PD}r_1^2P_l} &\approx -\phi_e\phi_n\rho_{A0}\left(\rho_{Bn}S_{n\psi_B} + \alpha S_n\right) + \phi_e\phi_n\left(\rho_{B0} + \alpha\right)\rho_{An}S_{n\psi_A} + \epsilon_e\epsilon_n\left(\rho_{B0} + \alpha\right)\rho_{An}C_{n\psi_A} \\ \frac{4V_X(t)}{\eta_M\eta_{PD}r_1^2P_l} &\approx \epsilon_e\phi_n\rho_{A0}\left(\rho_{Bn} - \alpha\right)S_{n\psi_B} + \phi_e\epsilon_n\rho_{A0}\left(\rho_{Bn}C_{n\psi_B} - \alpha C_n\right) \\ & \quad + \phi_e\epsilon_n\rho_{An}\left(\rho_{B0} - \alpha\right)C_{n\psi_A} - \epsilon_e\phi_n\rho_{An}\left(\rho_{B0} - \alpha\right)S_{n\psi_A}.\end{aligned}$$

We now test the most relevant cases for the main text.

### 3.1 Case 1: Frequency noise only, ideal EOM, cavity resonant with carrier

For the case of only frequency noise, an ideal phase modulator, and the cavity resonant only with the carrier ($\epsilon_e \to 0$, $\epsilon_n \to 0$, $\rho_{Bn} \to 1$, $\rho_{B0} \to 1$ and $\psi_B \to 0$) these quadratures simplify to

$$\begin{aligned}V_Y(t) &\to \sqrt{\frac{P_lP_e}{8}}\eta_M\eta_{PD}r_1^2\phi_n\left(1 + \alpha\right)\left(\rho_{An}S_{n\psi_A} - \rho_{A0}S_n\right) \\ V_X(t) &\to 0.\end{aligned}$$

where we have identified the power in each EOM-driven sideband $\sqrt{P_e} \approx \sqrt{\frac{1}{2}P_l}\phi_e$ from Eq. 6. The "amplitude" quadrature $V_X$ is zero to lowest order, which is sensible, since the laser is exactly on resonance and we are only modulating its frequency. With both sidebands present ($\alpha = 1$), the "phase" quadrature $V_Y$ also provides the dynamic response of the classic PDH error signal

$$V_Y = \sqrt{\frac{P_lP_e}{2}}\eta_M\eta_{PD}r_1^2\phi_n\left(\rho_{An}S_{n\psi_A} - \rho_{A0}S_n\right).$$

If the lower sideband is *not* present, the signal is simply a factor of 2 smaller; the "classic" PDH error signal receives a contribution from both sidebands in proportion to the frequency noise.

Now that all the nonlinear operations (photodiode, mixer) are complete, we have a linear mapping from the original noise $\Omega(t)$ to the error signal $V_Y$. We can convert this into a complex transfer function by noting that $V_Y$ is the real part of

$$\tilde{V}_Y = -i\sqrt{\frac{P_lP_e}{2}}\eta_M\eta_{PD}r_1^2\phi_n\left(\rho_A(\omega_n)e^{i\omega_n t} - \rho_A(0)e^{i\omega_n t}\right)$$

and that $\Omega$ is the real part of

$$\tilde{\Omega} = \Omega_n e^{i\omega_n t}.$$

The complex transfer function is then the ratio

$$\frac{\tilde{V}_Y}{\tilde{\Omega}} = \frac{\sqrt{2P_lP_e}\eta_M\eta_{PD}r_1^2t_1^2c\tau^2/L}{1 + i2\tau\omega_n} = \frac{2\phi_eE_l^2\beta\tau^2}{1 + i2\tau\omega_n}.$$

where we have used the definitions of $\phi_n$ from Eq. 4 and $\rho_A$ from Eq. 7 and defined $\beta = \eta_M\eta_{PD}r_1^2t_1^2c/2L$. The cavity acts as a low-pass filter.

### 3.2 Case 2: Frequency noise only, ideal EOM, cavity resonant with upper sideband

For the case of only frequency noise, a perfect phase modulator, and the cavity resonant with the upper sideband, $\epsilon_e \to 0$, $\epsilon_n \to 0$, $\rho_{An} \to 1$, $\rho_{A0} \to 1$ and $\psi_A \to 0$, and

$$\begin{aligned} V_Y(t) &\to -\sqrt{\frac{P_l P_e}{8}}\eta_M \eta_{PD} r_1^2 \phi_n \left(\rho_{Bn} S_{n\psi_B} - \rho_{B0} S_n\right) \\ V_X(t) &\to 0 \end{aligned}$$

and

$$\frac{\tilde{V}_Y}{\tilde{\Omega}} = -\sqrt{\frac{P_l P_e}{2}} \frac{\eta_M \eta_{PD} c\tau^2 r_1^2 t_1^2 / L}{1 + i2\tau\omega_n} = -\frac{\phi_e E_l^2 \beta \tau^2}{1 + i2\tau\omega_n}.$$

The error signal behaves exactly the same, but is half as large and inverted. The lower sideband does not play a role.

### 3.3 Case 3: Amplitude noise only, ideal EOM, cavity resonant with carrier

For the case of amplitude noise (still assuming a perfect phase modulator) and the cavity resonant with the carrier, $\epsilon_e, \phi_n \to 0$, $\rho_{Bn}, \rho_{B0} \to 1$, $\psi_B \to 0$, and the quadratures become

$$\begin{aligned} V_Y(t) &\to 0 \\ V_X(t) &\to \sqrt{\frac{P_l P_e}{8}}\eta_M \eta_{PD} r_1^2 \epsilon_n (1-\alpha)\left(\rho_{A0} C_n + \rho_{An} C_{n\psi_A}\right) \end{aligned}$$

The "phase" quadrature $V_Y$ is zero, as expected, regardless of the presence of the lower sideband. This is consistent with the notion that changing the laser's amplitude will not affect location of the error signal's zero-crossing. The "amplitude" quadrature $V_X$ in this case is the real part of

$$\begin{aligned} \tilde{V}_X &= \sqrt{\frac{P_l P_e}{8}}\eta_M \eta_{PD} r_1^2 \epsilon_n (1-\alpha)\left(\rho_A(0) + \rho_A(\omega_n)\right) e^{i\omega_n t} \\ &= \sqrt{\frac{P_l P_e}{8}}\eta_M \eta_{PD} r_1^2 \epsilon_n (1-\alpha) 2 \left(1 - \frac{c\tau t_1^2}{L}\left(1 - \frac{i\tau\omega_n}{1 + i2\tau\omega_n}\right)\right) e^{i\omega_n t} \end{aligned}$$

and

$$\frac{\tilde{V}_X}{\tilde{\epsilon}} = \sqrt{\frac{P_l P_e}{2}}\eta_M \eta_{PD} r_1^2 (1-\alpha)\left(1 - \frac{c\tau t_1^2}{L}\left(\frac{1 + i\tau\omega_n}{1 + i2\tau\omega_n}\right)\right).$$

This signal is only nonzero if the lower sideband is either missing or is otherwise not identical to the upper sideband ($\alpha \neq 1$).

### 3.4 Case 4: Amplitude noise only, ideal EOM, cavity resonant with upper sideband

If the cavity is instead resonant with the upper sideband, $\epsilon_e, \phi_n \to 0$, $\rho_{An}, \rho_{A0} \to 1$, $\psi_A \to 0$. Amplitude noise results in

$$\begin{aligned} V_Y(t) &\to 0 \\ V_X(t) &\to \sqrt{\frac{P_l P_e}{8}}\eta_M \eta_{PD} r_1^2 \epsilon_n \left(\rho_{\mathrm{Bn}} C_{n\psi_B} + \rho_{\mathrm{B0}} C_n - 2\alpha C_n\right) \end{aligned}$$

so

$$\tilde{V}_X = \sqrt{\frac{P_l P_e}{8}}\eta_M \eta_{PD} r_1^2 \epsilon_n \left(\rho_B(\omega_n) + \rho_B(0) - 2\alpha\right) e^{i\omega_n t}$$

and

$$\frac{\tilde{V}_X}{\tilde{\epsilon}} = \sqrt{\frac{P_l P_e}{2}}\eta_M \eta_{PD} r_1^2 \left(1 - \alpha - \frac{c\tau t_1^2}{L}\left(\frac{1+i\tau\omega_n}{1+i2\tau\omega_n}\right)\right)$$

with an overall offset determined by the lower sideband $\alpha$. The presence of the lower sideband ($\alpha = 1$) produces a PI-like behavior (see main text Eq. 5)

$$\frac{\tilde{V}_X}{\tilde{\epsilon}} = -\phi_e E_l^2 \beta\tau \left(\frac{1+i\tau\omega_n}{1+i2\tau\omega_n}\right).$$

# 4 Transfer from VCO input to error signal

When we measure the transfer function, we inject noise into the VCO, which is not quite the same as adding laser noise, since the VCO signal is also used as the local oscillator (LO) for the mixers. To ensure this does not impact our measurement, we now follow the same analysis above, keeping the VCO's extra components (again to second order) for the mixing stage.

Suppose the VCO has a modulated signal on its input

$$V_{in}(t) = V_n C_n$$

as is the case for our measurement of the closed-loop transfer function. The instantaneous frequency of the VCO's output voltage

$$\partial_t \phi_{LO}(t) = \omega_e + \eta_{VCO} V_n C_n$$

where $\eta_{VCO}$ is the VCO's conversion factor (units of Hz/V), and the phase is

$$\begin{aligned} \phi_{LO}(t) &= \omega_e t + \phi_n S_n \\ \phi_n &\equiv \frac{\eta_{VCO} V_n}{\omega_n} \end{aligned}$$

and its output voltage is

$$V_{out}(t) = V_e \sin(\omega_e t + \phi_n S_n).$$

If this voltage is sent to an EOM through which a "clean" laser at frequency $\omega_l$ passes, the output field will be

$$\begin{aligned} E(t) &= \sqrt{P_l}\cos\left(\omega_l t + \phi_e \sin(\omega_e t + \phi_n S_n)\right) \\ \phi_e &\equiv \eta_{EOM} V_e \end{aligned}$$

where the EOM's conversion efficiency $\eta_{EOM}$ has units of rad/V. Expanding to second order in $\phi$,

$$\begin{aligned} \frac{E(t)}{\sqrt{P_l}} &\approx C_l - S_l \phi_e \sin(\omega_e t + \phi_n S_n) - \frac{1}{2} C_l \phi_e^2 \sin^2(\omega_e t + \phi_n S_n) \\ &\approx C_l - S_l \phi_e \left[S_e + \phi_n C_e S_n\right] - \frac{1}{2} C_l \phi_e^2 \left[\frac{1}{2} - \frac{1}{2}\cos(2\omega_e t + 2\phi_n S_n)\right] \\ &\approx \left(1 - \frac{1}{4}\phi_e^2\right) C_l - \phi_e S_l S_e - \phi_e \phi_n S_l C_e S_n + \frac{1}{4}\phi_e^2 C_l C_{2e} \\ &= \left(1 - \frac{1}{4}\phi_e^2\right) C_l - \frac{1}{2}\phi_e \left[C_{l-e} - C_{l+e}\right] \\ &\quad -\frac{1}{4}\phi_e \phi_n \left[C_{l-e-n} - C_{l+e+n} - C_{l-e+n} + C_{l+e-n}\right] + \frac{1}{8}\phi_e^2 \left[C_{l-2e} + C_{l+2e}\right] \end{aligned}$$

Suppose this lands on a cavity of reflectivity (see 1)

$$r(\omega) \approx -r_1 \left(1 - \frac{t_1^2 \tau c/L}{1 + i2\tau\delta}\right) \equiv -r_1 \rho(\omega),$$

having a resonance centered on the upper sideband at $\omega_l + \omega_e$. The reflected field is then

$$\begin{aligned}
\frac{-E(t)}{r_1\sqrt{P_l}} &= \left(1 - \frac{1}{4}\phi_e^2\right) C_l + \frac{1}{2}\phi_e \left[-C_{l-e} + \rho_0 C_{l+e}\right] \\
&\quad + \frac{1}{4}\phi_e\phi_n \left[-C_{l-e-n} + \rho_n C_{l+e+n\psi} + C_{l-e+n} - \rho_n C_{l+e-n\psi}\right] + \frac{1}{8}\phi_e^2 \left[C_{l-2e} + C_{l+2e}\right].
\end{aligned}$$

If this lands on a photodiode it will generate a signal

$$\begin{aligned}
\frac{V_{PD}(t)}{\eta_{PD} r_1^2 P_l} &= \ldots + C_l\phi_e \left[-C_{l-e} + \rho_0 C_{l+e}\right] + \frac{1}{4}C_l\phi_e^2 \left[C_{l-2e} + C_{l+2e}\right] + \frac{1}{4}\phi_e^2 \left[\rho_0 C_{l+e} - C_{l-e}\right]^2 \\
&\quad + \frac{1}{2}\phi_e\phi_n C_l \left[-C_{l-e-n} + \rho_n C_{l+e+n\psi} + C_{l-e+n} - \rho_n C_{l+e-n\psi}\right] \\
&= \ldots + \frac{1}{2}\phi_e \left(\rho_0 - 1\right) C_e + \frac{1}{4}\phi_e^2 \left(1 - \rho_0\right) C_{2e} \\
&\quad + \frac{1}{4}\phi_e\phi_n \left[\rho_n C_{e+n\psi} - C_{e+n} + C_{e-n} - \rho_n C_{e-n\psi}\right]
\end{aligned}$$

If this signal lands on the signal port of the mixer, with the VCO output on the LO, it will be multiplied by

$$\begin{aligned}
V_{out}(t) &= \sin(\omega_e t + \phi_n S_n) \\
&\approx \left(S_e + \frac{1}{2}\phi_n \left[S_{e+n} - S_{e-n}\right]\right)
\end{aligned}$$

keeping only low frequency terms to produce the error signal:

$$\frac{4V_Y(t)}{\eta_M \eta_{PD} r_1^2 P_l} = \phi_e\phi_n \left[\left(\rho_0 - 1\right) S_n + S_n - \rho_n S_{n\psi}\right]$$

which is the real part of

$$\tilde{V}_Y(t) = -i\frac{P_l}{4}\phi_e\phi_n\eta_M\eta_{PD} r_1^2 \left[\rho(0) - \rho(\omega_n)\right] e^{i\omega_n t}$$

where $\beta$ is some proportionality constant that depends on the laser power and the efficiencies of the VCO, photodiode, and mixer. The transfer function from the input to the error signal is then

$$\begin{aligned}
\frac{\tilde{V}_Y}{\tilde{V}_{in}} &= -i\frac{P_l}{4}\phi_e\eta_{VCO}\eta_M\eta_{PD} r_1^2 \frac{\left[\rho(0) - \rho(\omega_n)\right]}{\omega_n} \\
&= -\sqrt{\frac{P_l P_e}{2}} \frac{\eta_{VCO}\eta_M\eta_{PD} c\tau^2 r_1^2 t_1^2/L}{1 + i2\tau\omega_n} \\
&= -\eta_{VCO}\frac{\phi_e E_l^2 \beta\tau^2}{1 + i2\tau\omega_n}
\end{aligned}$$

Which apart from $\eta_{VCO}$ is the same as the laser noise transfer function of the previous section (case 2) and similarly $V_X(t) \to 0$. This means that, despite the modulated frequency sent to the LO port of the mixer, the method described in the text still measures the correct transfer function of the VCO, EOM, cavity, diode, and demodulation circuit.

## 5 Error signal for wider range of VCO outputs

Figure 1 shows the two quadrature amplitudes of the photodiode signal, taken with a shorter cavity of $L = 5$ cm and for a wider range of VCO tune voltages than that of Fig. 2(c) in the main text. Over this range, the non-ideal response of the system components is visible (see in particular the peaks of $V_X(\delta)$, which systematically vary in amplitude with VCO frequency). Large frequency noise will therefore produce amplitude noise even if it is perfectly tracked by a sideband. This highlights the fact that, while a large headroom is desirable to remain locked in the presence of large fluctuations, it is always preferable to engineer a stable, vibration-isolated cavity.

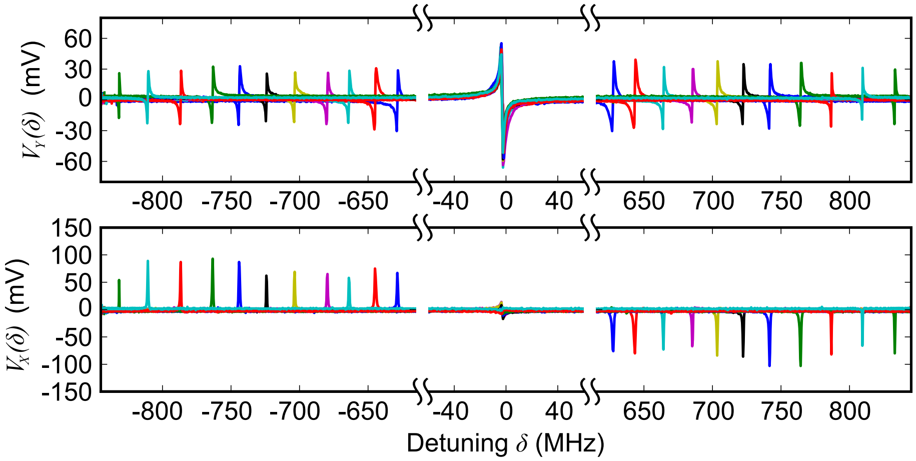


Figure 1: Quadrature amplitudes of the photodiode signal for 11 different VCO voltages.
